# Supplementary material for: Spectral alignment of single-photon emitters in diamond using strain gradient
Source: arXiv:1807.06991 ancillary file (2018-07-18)
Supplement: Supplementary file 1 [file gev-supp.pdf]

# Spectral alignment of single-photon emitters in diamond using strain gradient

## *Supplemental Materials*

Smarak Maity,[1,*] Linbo Shao,[1,†] Young-Ik Sohn,[1] Srujan Meesala,[1] Bartholomeus Machielse,[1] Edward Bielejec,[2] Matthew Markham,[3] and Marko Lončar[1]

[1] *John A. Paulson School of Engineering and Applied Sciences, Harvard University, 29 Oxford Street, Cambridge, MA 02138, USA*
[2] *Sandia National Laboratories, Albuquerque, NM 87185, USA*
[3] *Element Six Global Innovation Centre, Fermi Avenue, Harwell Oxford, Didcot, Oxfordshire OX110QR, United Kingdom*

### A. Device Fabrication

The diamond samples used in this work are electronic grade single crystal diamonds from Element Six (Element Six Technologies US Corporation, Santa Clara, CA) synthesized by chemical vapor deposition. The top face of the diamond sample is (001), and the edges are oriented along the ⟨110⟩ directions. The detailed fabrication processes are as follows. (1) The patterns of microcantilevers are defined by electron-beam lithography on the diamond surface. (2) The microcantilevers are fabricated by top-down oxygen reactive-ion etching and angled ion beam milling. (3) The Ge atoms are deterministically implanted at desired sites by a focused beam of 200 keV $^{74}Ge^{2+}$ ions. (4) The sample is annealed under high vacuum at 800°C for 12 hours and 1100°C for 2 hours. (5) The electrodes are patterned by electron-beam lithography and deposited by electron beam evaporation of a 10 nm thick titanium layer followed by a 200 nm thick layer of gold; unwanted metals are removed by solvent lift-off.

* These authors contributed equally.
† These authors contributed equally.
shaolb@seas.harvard.edu

### B. Local Coordinate System of GeVs

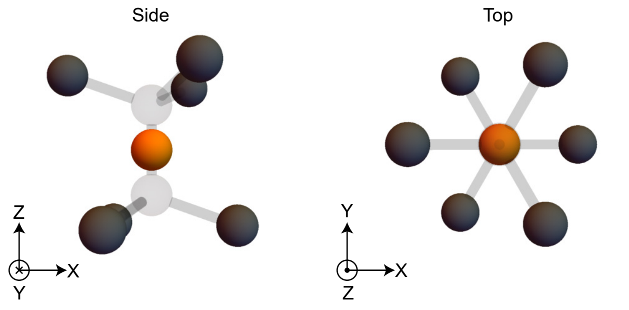


FIG. S1. Side and top views of the molecular structure of the GeV center, showing the local coordinate system of GeV used to specify the strain tensor components. Orange, black, and grey spheres represent germanium, carbon, and vacancy.

### C. Electronic energy levels of the GeV center under strain

The GeV has the same $D_{3d}$ symmetry as the silicon vacancy color center, so group theoretic arguments predict a qualitatively similar strain Hamiltonian for both. The ground and excited states of the GeV are 4-fold degenerate, each made up of 4 states in the direct product space of the orbital $\{|e_X\rangle, |e_Y\rangle\}$ and spin $\{|\uparrow\rangle, |\downarrow\rangle\}$ bases. In the absence of strain, spin-orbit coupling splits both the ground and excited states into pairs of 2 degenerate eigenstates with the Hamiltonian

$$\mathcal{H}^{\mathrm{SO}} = -\frac{\lambda_{\mathrm{SO}}}{2}\begin{bmatrix}0 & i\\ -i & 0\end{bmatrix}\otimes\begin{bmatrix}1 & 0\\ 0 & -1\end{bmatrix} \qquad \text{(S1)}$$

These pairs of degenerate eigenstates generate the 4 optical transitions that are visible as peaks in the photoluminescent spectrum of the GeV. Strain is a 9-component tensor $\epsilon_{ij}$, and the strain Hamiltonian is expressed in terms of the quantities $\alpha, \beta, \gamma$ which are linear combinations of the strain tensor components multiplied by strain

susceptibility constants.

$$\mathcal{H}^{\text{strain}} = \begin{bmatrix} \alpha-\beta & \gamma \\ \gamma & \alpha+\beta \end{bmatrix} \otimes \begin{bmatrix} 1 & 0 \\ 0 & 1 \end{bmatrix} \tag{S2}$$

$$\alpha = t_\perp(\epsilon_{XX}+\epsilon_{YY}) + t_\parallel \epsilon_{ZZ} \tag{S3}$$

$$\beta = d(\epsilon_{XX}-\epsilon_{YY}) + f\epsilon_{ZX} \tag{S4}$$

$$\gamma = -2d\epsilon_{XY} + f\epsilon_{YZ} \tag{S5}$$

By diagonalizing the total Hamiltonian $\mathcal{H}^{\text{SO}} + \mathcal{H}^{\text{strain}}$ we once again get pairs of 2 degenerate eigenstates in the ground and excited states each, with energies

$$E_{1,2} = \alpha \pm \sqrt{\left(\frac{\lambda_{\text{SO}}}{2}\right)^2 + \beta^2 + \gamma^2} \tag{S6}$$

These can be related to the positions of the 4 spectral lines as

$$\bar{\nu} = \bar{\nu}_0 + (\alpha_e - \alpha_g) \tag{S7}$$

$$\Delta_g = \sqrt{\lambda_{\text{SO},g}^2 + 4(\beta_g^2 + \gamma_g^2)} \tag{S8}$$

$$\Delta_e = \sqrt{\lambda_{\text{SO},e}^2 + 4(\beta_e^2 + \gamma_e^2)} \tag{S9}$$

where $\Delta_{g,e}$ are the ground and excited state splittings, and $\bar{\nu}$ is the mean frequency of the 4 lines. By fitting the observed spectral lines for both classes of GeVs to these expressions with the strain tensor components calculated with a finite element simulation, we estimate the strain susceptibility constants of the GeV.

### D. Experimental details

Low temperature experiments are performed in a continuous flow liquid helium cryostat (Janis ST-500). The devices are addressed with a home built confocal microscope that scans an excitation laser across the sample, while simultaneously collecting the emitted photons in a different wavelength range. The collected photons can be sent to an avalanche photo diode (APD) for photon counting or a spectrometer.

**Photoluminescence measurements** These measurements are related to data in Figs. 1(c) and 2. All four (4) transitions are visible in off-resonant excitation at the operating temperature of 50 K. The GeV centers are excited by a 532 nm laser and photons near the 602 nm zero phonon line (ZPL) are selected by a band pass filter. At the excitation power of about 1 mW, we typically get $3 \times 10^4$ photon counts per second (cps) from a single GeV. The spectra of the collected photons are recorded by the spectrometer (Horiba iHR550).

A high voltage DC source (SRS PS310) is used to apply a potential between the electrodes and hence introduce strain in the cantilever. We slowly ramp the voltage to bend the cantilever and take spectral measurements at intermediate voltages. The maximum voltage we can apply is limited to 250 V due to high current observed through the device.

**Resonant excitation measurements** These measurements are related to data in Figs. 1(d), 3 and 4. The measurements are performed at a temperature of 10 K, minimizing the thermal broadening of the spectral lines. The GeVs are excited resonantly with a tunable probe laser near 602 nm, and emitted photons at the phonon side band (PSB) $>$ 610 nm are selected by a optical long-wavelength pass filter. The 602 nm tunable probe laser is home built, using sum frequency generation to mix light from a 980 nm laser diode and a 1550 nm tunable laser in a $\chi^{(2)}$ nonlinear crystal (40 mm MgO:PPLN). The probe laser is scanned across the optical transitions of the GeV while its wavelength is monitored with a high resolution wavemeter. The recorded PSB fluoresence counts allow us to measure a high resolution spectrum.

**Autocorrelation measurements** The second order autocorrelation ($g^{(2)}$) of the collected photons is measured in the resonant excitation configuration by sending the photons into two APDs using a fiber beam splitter. The electrical pulses from the APDs are sent to a time correlated single photon counter (TCSPC) with a resolution of 32 ps.
